# Supplementary material for: Field free switching through bulk spin-orbit torque in L10-FePt films deposited on vicinal substrates
Source: arXiv:2203.06921 source file (2022-03-14)
Supplement: Supplementary file 1 [file supplementary_information_1.pdf]

# Supplementary information

**Field free switching through bulk spin-orbit torque in $L1_0$-FePt films deposited on vicinal substrates**

*Yongming Luo[1]*,Yanshan Zhuang[1],Zhongshu Feng[1],Haodong Fan[1],Birui Wu[1],Menghao Jing[1], Ziji Shao[1],Hai Li[1],Ru Bai[1], Yizheng Wu[2], Ningning Wang[1] and Tiejun Zhou[1]**

[1] Center for Integrated Spintronic Devices, Hangzhou Dianzi University, Hangzhou, Zhejiang, 310018, People's Republic of China.

[2] State Key Laboratory of Surface Physics and Department of Physics, Fudan University, Shanghai 200433, People's Republic of China.

## 1. SOT switching of the $L1_0$-FePt grown on flat substrates.

**Figure S1.** Current-induced magnetization switching of the 6 nm $L1_0$-FePt grown on flat MgO substrates, with different fields applied along X direction.

## 2. SOT switching of the $L1_0$-FePt when current is applied in the y direction.

**Figure S2**. Current-induced magnetization switching of the 6 nm $L1_0$-FePt grown on vicinal substrate (α=7°), with current applied in the y direction. No field-free switching could be realized. The switching could happen when Hy is applied.

## 3. Field free switching of the $L1_0$-FePt film with different thickness.

**Figure S3.** Current-induced magnetization switching of the $L1_0$-FePt films with different thickness. $L1_0$-FePt grown on vicinal substrate (α=7°). No field is applied. The critical switching current density Jc decrease with the increasing film thickness.

## 4. Micro-magnetization Simulation

We performed micro-magnetization simulation to verify the rotational symmetry of the AMR signals and the field free SOT switching of the FePt magnetization, by using OOMMF. In our simulation model, we choose a FePt film with 200 nm x 50 nm x 6 nm (length x width x thickness) in size, the unit cell size is 5 nm x 5 nm x 6 nm. In our simulation, the magnetic parameters of FePt is as follows: the stiffness of FePt: A=9e-12 J/m; saturation magnetization: Ms=1.2e5 A/m; the perpendicular anisotropy is Ku=1e5 J/m^3. Damping α=0.01. We compare the simulation results with perpendicular and titled anisotropies, the results are shown in **Figure S4**. The simulation shown that film with perpendicular anisotropy could not realize field free switching. **Figure S4**a. To realize field free switching with tilted anisotropy, the current direction should be perpendicular with the tilting direction of the anisotropy (see **Figure. 4**c), if the current direction is colinear with the tilting direction of the anisotropy, one could not realize field free switching, see **Figure 4**b. Which is consistence with our experiment results. Besides, our simulation shown that when current is colinear with the tilting direction, the switching loop would be asymmetric (shift to -x direction,), the shift would decrease with the increasing amplitudes of Hx. In our experiment, we found such asymmetry is small, this may be due to the discrepancy of magnetic parameters between the simulation and the experiments.

**Figure S4.** Simulation of the current induced switching of FePt magnetization, with different anisotropy directions. (a) Perpendicular anisotropy. (b) Easy axis tilted in the xz plane, with tilting angle $\varphi_{xz} = 8^\circ$. (c) Easy axis tilted in the yz plane, with tilting angle $\varphi_{yz} = 8^\circ$. In each figure, the direction of easy axis, current direction, and field direction are schematically shown in the top panel, and the simulation results are shown in the bottom panel.

## 5. Spin orbit torque induced effective fields as a function of the current amplitudes.

**Figure S5.** $\Delta H_{L(T)}$ as a function of the current amplitudes. The “+”(“-”) represent results obtained from upward (downward) initial FePt magnetization, respectively.
